# Supplementary material for: Minimal Variance Sampling with Provable Guarantees for Fast Training of Graph Neural Networks
Source: arXiv:2006.13866 source file (2021-09-05)
Supplement: Supplementary file 1 [file bandit_sampling.tex]

\section{Approximate importance sampling using bandit sampling}\label{appendix:batch_mab_sample}

\begin{lemma} \label{lemma:vars_convex}
Let $\boldsymbol{p}_t^\star$ be the optimal solution and $\boldsymbol{p}_t$ be the approximate solution at step $t$.  
	For any real value constant $\eta \leq 1$ and any valid distributions $\boldsymbol{p}_t$ and $\boldsymbol{p}_t^\star$ we have
	\begin{equation*}
	(1-2\eta) \mathbb{G}\left(\boldsymbol{p}_t\right) - (1-\eta) \mathbb{G}\left(\boldsymbol{p}_t^\star\right) \leq \langle \boldsymbol{p}_t - \boldsymbol{p}_t^\star, \nabla \mathbb{G}\left(\boldsymbol{p}_t\right) \rangle + \eta \langle \boldsymbol{p}_t^\star,\nabla \mathbb{G}\left(\boldsymbol{p}_t\right) \rangle.
	\end{equation*}
\end{lemma}

\begin{proof} [Proof of Lemma \ref{lemma:vars_convex}]
	The function $\mathbb{G}\left(\boldsymbol{p}\right)$ is convex with respect to $\boldsymbol{p}$, hence for any two  $\boldsymbol{p}_t$ and $\boldsymbol{p}_t^\star$ we have
	\begin{equation*}
	\mathbb{G}(\boldsymbol{p}_t) - \mathbb{G}(\boldsymbol{p}_t^\star) \leq \langle \boldsymbol{p}_t-\boldsymbol{p}_t^\star, \nabla \mathbb{G}(\boldsymbol{p}_t)  \rangle.
	\end{equation*}
	Multiplying both sides of this inequality by $1-\eta$, and using that $\langle \boldsymbol{p}_t, \nabla \mathbb{G}(\boldsymbol{p}_t)  \rangle = -\mathbb{G}(\boldsymbol{p}_t)$ we have
	\begin{equation*}
	\begin{aligned}
	(1-\eta) \mathbb{G}(\boldsymbol{p}_t) - (1-\eta) \mathbb{G}(\boldsymbol{p}_t^\star) &\leq  \langle \boldsymbol{p}_t-\boldsymbol{p}_t^\star, \nabla \mathbb{G}(\boldsymbol{p}_t)  \rangle -\eta \langle \boldsymbol{p}_t-\boldsymbol{p}_t^\star, \nabla \mathbb{G}(\boldsymbol{p}_t)  \rangle \\& =
	\langle \boldsymbol{p}_t-\boldsymbol{p}_t^\star, \nabla \mathbb{G}(\boldsymbol{p}_t)  \rangle +\eta \langle \boldsymbol{p}_t^\star, \nabla \mathbb{G}(\boldsymbol{p}_t)  \rangle + \eta \mathbb{G}(\boldsymbol{p}_t),
	\end{aligned}
	\end{equation*}
	which concludes the proof.
\end{proof}

\todo{there are bugs in terms of $b$ need to be fixed }
\batchmabsample
\begin{proof} [Proof of Lemma \ref{lemma:batch_mab_sample}]
    For the ease of presentation, we denote $\hat{G}_{i,t}$ the upper bound of the gradient norm of $i$-th data point at time $t$, denote $a_{i,t} = \hat{G}_{i,t}^2/n^2$ and the potential function $W_t = \sum_{i=1}^n w_{i,t}$.
	The proof is based on upper bounding and lower bounding the potential function $W_T$ at final iteration $T$. 
	
	We first derive the lower bound.
	Let $r_{i,t} = a_{i,t}/p_{i,t}^2$ be the reward of data point $i$ and $\hat{r}_{i,t}  =r_{i,t}\cdot\mathbf{1}_{\{I_t=i\}}/p_{i,t}$ be an unbiased estimator for $r_{i,t}$. Then, the update rule of weight $w_{i,t}$ is $w_{i,t+1}=w_{i,t}\cdot\exp(\delta\hat{r}_{i,t})$.
	Therefore, $w_{i,t}=\exp\left(\delta\sum_{t=1}^{T}\hat{r}_{i,t}\right)$ and the potential function $W_T= \sum_{i=1}^{n} w_{i,T} \geq  w_{j,t}=\exp\left(\delta\sum_{t=1}^{T}\hat{r}_{j,t}\right)$ for all $j=1,\cdots,n$. Knowing that $W_1=\sum_{i=1}^{n} w_{i,1}=n$,
	we get the following lower bound for the potential function $W_T$,
	\begin{equation}\label{eq:lower}
	\delta \sum_{t=1}^{T} \hat{r}_{j,t} - \ln n \leq \ln\frac{W_T}{W_1}.
	\end{equation}
	
	Then, let us upper bound $W_T$. By the definition of potential function $W_t$ and the update rule, we have
	\begin{equation*}
	\frac{W_{t+1}}{W_t} = \frac{\sum_{i=1}^{n}w_{i,t+1}}{W_t} = \frac{\sum_{i=1}^{n}w_{i,t} \exp(\delta \hat{r}_{i,t})}{W_t} = \sum_{i=1}^{n} \left(\frac{p_{i,t}-\eta/n}{(1-\eta)}\right) \exp(\delta \hat{r}_{i,t}).
	\end{equation*}
	
	Using the inequality that $\exp(x) < 1+x+x^2$ which hold for all $x<1$, we have
	\begin{equation*} 
	\begin{aligned}
	\frac{W_{t+1}}{W_t} \leq \sum_{i=1}^{n} \left(\frac{p_{i,t}-\eta/n}{(1-\eta)}\right) \left(1+\delta \hat{r}_{i,t}+(\delta \hat{r}_{i,t})^2\right) &\leq 1+ \frac{\delta}{(1-\eta)}\sum_{i=1}^{n}p_{i,t} \hat{r}_{i,t} + \frac{\delta^2}{(1-\eta)}\sum_{i=1}^{n}p_{i,t} \hat{r}_{i,t}^2. 
	\end{aligned}
	\end{equation*} 
	
	Note that the above inequality hold when $\delta \hat{r}_{i,t}<1$, we leave this later after we get the optimal $\delta$.
	Using the inequality $\ln (1+x)\leq x$ which holds for all $x\geq
	0$ we get
	\begin{equation*}
	\ln \frac{W_{t+1}}{W_t} \leq \frac{\delta}{(1-\eta)} \sum_{i=1}^{n}p_{i,t} \hat{r}_{i,t} + \frac{\delta^2}{(1-\eta)}\sum_{i=1}^{n}p_{i,t} \hat{r}_{i,t}^2.
	\end{equation*}
	Sum above equation for $t = 1,\cdots,T$, we get the following telescopic sum 
	\begin{equation} \label{eq:upper}
	\sum_{t=1}^{T}\ln \frac{W_{t+1}}{W_t} = \ln \frac{W_T}{W_1}  \leq \frac{\delta}{(1-\eta)} \sum_{t=1}^{T}\sum_{i=1}^{n}p_{i,t} \hat{r}_{i,t} + \frac{\delta^2}{(1-\eta)} \sum_{t=1}^{T} \sum_{i=1}^{n}p_{i,t} \hat{r}_{i,t}^2.
	\end{equation}
	
	Combining the lower bound in Equation~\ref{eq:lower} and the upper bound in Equation~\ref{eq:upper}, we get
	\begin{equation*}
	\delta\sum_{t=1}^{T} \hat{r}_{j,t} - \ln n \leq \frac{\delta}{(1-\eta)} \sum_{t=1}^{T}\sum_{i=1}^{n}p_{i,t} \hat{r}_{i,t} + \frac{\delta^2}{(1-\eta)}\sum_{t=1}^{T}\sum_{i=1}^{n}p_{i,t} \hat{r}_{i,t}^2.
	\end{equation*}
	Given $\boldsymbol{p}_t$ we have $\cE[\hat{r}_{i,t}^2]  = r_{i,t}^2/p_{i,t}$, 
	hence, taking expectation on both side, we have
	\begin{equation*}
	\delta \sum_{t=1}^{T} r_{j,t} - \ln n \leq \frac{\delta}{(1-\eta)} \sum_{t=1}^{T}\sum_{i=1}^{n}p_{i,t} r_{i,t} + \frac{\delta^2}{(1-\eta)}\sum_{t=1}^{T}\sum_{i=1}^{n}r_{i,t}^2.
	\end{equation*}
	
	Using the fact that $\sum_{j=1}^n p^\star_{j,t} = 1$, we replace the left hand side as
	\begin{equation*}
	\delta\sum_{t=1}^{T} \sum_{j=1}^{n} p^\star_{j,t}r_{j,t} - \ln n \leq \frac{\delta}{(1-\eta)} \sum_{t=1}^{T}\sum_{i=1}^{n}p_{i,t} r_{i,t} + \frac{\delta^2}{(1-\eta)}\sum_{t=1}^{T}\sum_{i=1}^{n}r_{i,t}^2,
	\end{equation*}
	
	Multiply both side by $(1-\eta)/\delta$ we have
	\begin{equation*}
	(1-\eta)\sum_{t=1}^{T} \sum_{j=1}^{n} p^\star_{j,t}r_{j,t} - \frac{(1-\eta)}{\delta}\ln n \leq \sum_{t=1}^{T}\sum_{i=1}^{n}p_{i,t} r_{i,t} + \delta \sum_{t=1}^{T}\sum_{i=1}^{n}r_{i,t}^2,
	\end{equation*}
	
	As $r_{i,t}= a_{i,t}/p_{i,t}^2=-\nabla_i \mathbb{G}_t(\boldsymbol{p}_t)$, we have $\sum_{i=1}^{n} p_ir_{i,t} = - \langle \boldsymbol{p}, \nabla \mathbb{G}_t(\boldsymbol{p}_t) \rangle$ for any distribution $\boldsymbol{p}$, rearranging it, we find
	\begin{equation*} 
	\sum_{t=1}^{T} \langle \boldsymbol{p}_t-\boldsymbol{p}_t^\star, \mathbb{G}_t(\boldsymbol{p}_t) \rangle + \eta \sum_{t=1}^{T} \langle \boldsymbol{p}_t^\star, \mathbb{G}_t(\boldsymbol{p}_t) \rangle \leq \frac{1-\eta}{\delta}\ln n +  \delta \sum_{t=1}^{T} \sum_{i=1}^{n}r_{i,t}^2.
	\end{equation*}
	
	Using Lemma~\ref{lemma:batch_mab_sample} we have
	\begin{equation*} 
	(1-2\eta) \sum_{t=1}^{T} \mathbb{G}_t(\boldsymbol{p}_t) - (1-\eta) \sum_{t=1}^{T} \mathbb{G}_t(\boldsymbol{p}_t^\star) \leq
	\frac{1-\eta}{\delta}\ln n +  \delta \sum_{t=1}^{T} \sum_{i=1}^{n}r_{i,t}^2,
	\end{equation*}
	which yields
	\begin{equation*} 
	\sum_{t=1}^{T} \mathbb{G}_t(\boldsymbol{p}_t)  \leq \frac{1-\eta}{1-2\eta}  \sum_{t=1}^{T} \mathbb{G}(\boldsymbol{p}_t^\star) +
	\frac{1-\eta}{\delta (1-2\eta)}\ln n +  \frac{\delta}{1-2\eta} \sum_{t=1}^{T} \sum_{i=1}^{n}r_{i,t}^2.
	\end{equation*}
	Note that this gives an upper bound on $\sum_{t=1}^{T} \mathbb{G}_t(\boldsymbol{p}_t)$ only if $\eta < 0.5$.
	Finally, we know that $r_{i,t} \leq n^2a_{i,t}/\eta^2$. By setting $\eta = 0.4$ and $\delta=\sqrt{\eta^4 \ln n/(T\sum_{i=1}^n \hat{G}^2_i)}$, we conclude the first part of proof 
	\begin{equation*}
	\sum_{t=1}^{T} \mathbb{G}_t(\boldsymbol{p}_t)  \leq 3 \sum_{t=1}^{T} \mathbb{G}(\boldsymbol{p}_t^\star) +
	50 \sqrt{T\left(\sum_{i=1}^n \hat{G}^2_i\right) \ln n}  .
	\end{equation*}
	
	Therefore, to guarantee $\delta \hat{r}_{i,t}<1$, we have
	
\end{proof}
