# Supplementary material for: Minimal Variance Sampling with Provable Guarantees for Fast Training of Graph Neural Networks
Source: arXiv:2006.13866 source file (2021-09-05)
Supplement: Supplementary file 2 [file calculate_threshold.tex]

\section{Algorithm \texttt{CalculateProbs}}\label{appendix:calculate_probs}

\begin{algorithm2e}[H]
	\DontPrintSemicolon
    \caption{\texttt{CalculateProbs}($\mathbf{g}, n$)}
	\label{algorithm:calculate_probs}
	\textbf{input:} 
	A set of gradient $\mathbf{g} = (\mathbf{g}_1, \mathbf{g}_2, \cdots, \mathbf{g}_N)$ and desired number of samples $n$\\
    
    $\texttt{candidatesArray} = (\mathbf{g}_1,\mathbf{g}_2,\cdots,\mathbf{g}_N)$,~$\texttt{sampleSize} = n$,~ $\texttt{sumSmall}=0$,~ $\texttt{nLarge}=0$ \\
    $\mu = \texttt{CalculateThreshold}(\texttt{candidatesArray}, \texttt{sampleSize}, \texttt{sumSmall}, \texttt{nLarge})$ \\
    $p_i = \min(1, \mathbf{g}_i/\mu)$ for $i=1,\cdots,N$ \\
    
    \textbf{output:} 
    $\boldsymbol{p} = (p_1, p_2, \cdots, p_N)$
\end{algorithm2e}

\section{Algorithm \texttt{CalculateThreshold}}\label{appendix:calculate_thresh}

\begin{algorithm2e}[H]
	\DontPrintSemicolon
    \caption{\texttt{CalculateThreshold}(\texttt{candidatesArray}, \texttt{sampleSize}, \texttt{sumSmall}, \texttt{nLarge})}
 	\label{algorithm:calculate_thresh}
    $\texttt{candidate} = \texttt{candidatesArray}[0]$ \\
    $\texttt{smallArray} = \texttt{candidatesArray}[\texttt{candidatesArray} < \texttt{candidate}]$ \\
    $\texttt{largeArray} = \texttt{candidatesArray}[\texttt{candidatesArray} > \texttt{candidate}]$ \\
    $\texttt{equalArray} = \texttt{candidatesArray}[\texttt{candidatesArray} = \texttt{candidate}]$ \\
	\If{$\texttt{curSampleSize} < \texttt{sampleSize}$}{
	    \If{$len(\texttt{smallArray}) = 0$}{
	    \textbf{return} ~$\texttt{sumSmall}/(\texttt{sampleSize}-\texttt{nLarge}-len(\texttt{largeArray})-1)$ \\
	    }\Else{
	    $\texttt{nLarge} = \texttt{nLarge} + len(\texttt{largeArray})+len(\texttt{equalArray})$ \\
	    \textbf{return} ~$\texttt{CalculateThreshold}(\texttt{smallArray}, \texttt{sampleSize}, \texttt{sumSmall}, \texttt{nLarge})$
	    }
	}\Else{
	    \If{$len(\texttt{largeArray}) = 0$}{
	    \textbf{return} ~$(\texttt{sumSmall} + sum(\texttt{smallArray}) + sum(\texttt{equalArray}))/(\texttt{sampleSize}-\texttt{nLarge})$ \\
	    }\Else{
	    $\texttt{nLarge} = \texttt{nLarge} + len(\texttt{largeArray})+len(\texttt{equalArray})$ \\
	    \textbf{return} ~$\texttt{CalculateThreshold}(\texttt{largeArray}, \texttt{sampleSize}, \texttt{sumSmall}, \texttt{nLarge})$
	    }
	}
\end{algorithm2e}
