# Supplementary material for: Minimal Variance Sampling with Provable Guarantees for Fast Training of Graph Neural Networks
Source: arXiv:2006.13866 source file (2021-09-05)
Supplement: Supplementary file 3 [file compare_sota.tex]

\section{Compare with existing method}

\paragraph{Compare with VRGCN}
Since \texttt{MVS-GCN} and \texttt{MVS-GCN+} also uses variance reduction on embedding matrix, here we emphasize the key differences:
\begin{itemize}
    \item Our sampling method is 1-shot sampling, i.e., only need to sample one time to construct one mini-batch, while \texttt{VRGCN} requires samplers to travel recursively for each layer and each node in the mini-batch. 
    % \todo{ For example, on for a 5 layer GCN on PPI dataset with batch size $512$ and neighbor size $2$, it takes \texttt{MVS-GCN} $1.039s$ to construct mini-batch and $0.703$ for calculation while takes \texttt{VRGCN} $10.095$ to construct the mini-batch and $1.816s$ for calculation}.
    \item Our algorithm requires a constant number of nodes to calculate in each layer, while the number of nodes need for calculation grows exponentially with respect to the number of layers.
    \item Our algorithm requires multiply adjacency matrix with embedding matrix one time for each forward propagation, while \texttt{VRGCN} requires \footnote{Denote $\tilde{\mathbf{L}}$ as the stochastic Laplacian matrix of $\mathbf{L}$, and $\tilde{\mathbf{H}}$ as the history activation of $\mathbf{H}$. \texttt{VRGCN} need to estimate the embedding matrix. Although $\tilde{\mathbf{L}}\mathbf{H}$, $\tilde{\mathbf{L}}\bar{\mathbf{H}}$ can be integrated as $\tilde{\mathbf{L}}(\mathbf{H}-\bar{\mathbf{H}})$, it requires us to design specific graph convolution operation for \texttt{VRGCN}, which restrict its flexibility to generalize on to different backbones.}{at least} two times. Therefore, the computation cost of our algorithm is relatively lower, especially when the number of layers is large.
\end{itemize}

\paragraph{Compare with GraphSaint, ClusterGCN}
Since \texttt{MVS-GCN} and \texttt{MVS-GCN+} also uses subgraph sampling to construct mini-batch, here we emphasize the key differences:
\begin{itemize}
    \item Our sampling method use importance sampling based on the gradient of each data point to minimize the \footnote{Including embedding approximation variance and gradient approximation variance}{overall variance}, \texttt{GraphSaint} use importance sampling based on the Laplacian matrix to minimize the embedding approximation variance, while \texttt{ClusterGCN} do not apply any variance related analysis. Our sampling method has solid theoretical analysis showing that sampling based on gradient can minimize the overall variance.
    \item Node-wise subgraph sampling results in a sparse subgraph with high variance when the mini-batch size is small. 
    Our algorithms overcome the limitation by using historical activation of the previous layer to reduce variance, while \texttt{GraphSaint} overcome the limitation by using a huge mini-batch.
    \item Our sampling method and \texttt{GraphSaint} use 1-shot sampling to construct the mini-batch during training. \texttt{ClusterGCN} first partition graph into several clusters during pre-processing, and clusters are randomly selected to form the mini-batch, then a normalized Laplacian matrix is calculated based on the sampled clusters. 
\end{itemize}
