# Supplementary material for: Minimal Variance Sampling with Provable Guarantees for Fast Training of Graph Neural Networks
Source: arXiv:2006.13866 source file (2021-09-05)
Supplement: Supplementary file 4 [file convergence_analysis.tex]

\section{Convergence Analysis}\label{appendix:convergence_analysis}
The proof of Theorem \ref{theorem:sgcn_general_theorem} has the following steps:
\begin{itemize}
    \item We show in Lemma \ref{lemma:convergence_rate_general} that the convergence speed is a function of mean-square error  of the stochastic gradient estimator $\cE[\|\tilde{\mathbf{g}}_t-\nabla f(\boldsymbol{\theta}_t)\|^2]$
    \item We show in Lemma \ref{lemma:mse} that the mean-square error admits the following bias-variance decomposition $\cE[\|\tilde{\mathbf{g}}_t-\nabla f(\boldsymbol{\theta}_t)\|^2] = \cE_t[\|\tilde{\mathbf{g}}_t - \mathbf{g}_t\|^2] + \cE_t[\|\mathbf{g}_t - \nabla F(\boldsymbol{\theta}_t)\|^2]$, where $\cE[\tilde{\mathbf{g}}] = \mathbf{g}$
    \item We derive the upper-bound of $\cE_t[\|\tilde{\mathbf{g}}_t - \mathbf{g}_t\|^2]$ and $\cE_t[\|\mathbf{g}_t - \nabla F(\boldsymbol{\theta}_t)\|^2]$ respectively in Lemma \ref{lemma:grad_bias} and Lemma \ref{lemma:compare_vars}
    \item We combine the results above to conclude the proof for Theorem \ref{theorem:sgcn_general_theorem}.
\end{itemize}

%#######################################
%#########General Convergence ##########
% \begin{lemma}\label{lemma:convergence_rate_general}
% Suppose function $f(\boldsymbol{\theta}_t)$ has $L_f$-Lipschitz continuous gradient. The mean-square error (MSE) of stochastic gradient $\cE[\|\tilde{\mathbf{g}}_t-\nabla f(\boldsymbol{\theta}_t)\|^2] \leq \Delta$ is bounded by a constant $\Delta>0$. Set step size $\eta = \min\{\frac{1}{L_f}, \sqrt{\frac{\cE[f(\boldsymbol{\theta}_{1})] - \cE[f(\boldsymbol{\theta}_{*})]}{\Delta L_f T}}\}$ and let $\Tilde{\boldsymbol{\theta}} = \min_t \cE[\|\nabla f(\boldsymbol{\theta}_t)\|]$, we have
% \begin{equation*}
%     \cE[\|\nabla f(\Tilde{\boldsymbol{\theta}}_t)\|^2] \leq \sqrt{\frac{16L_f \Delta \left(\cE[f(\boldsymbol{\theta}_{1})] - \cE[f(\boldsymbol{\theta}_{*})]\right)}{T}}
% \end{equation*}
% \end{lemma}
\convergencerategeneral
\begin{proof} [Proof of Lemma \ref{lemma:convergence_rate_general}]
\todo{that proof also introduce a residual error $\Delta$. i change it using another way. result match \url{https://arxiv.org/pdf/1309.5549.pdf}}
By the assumption that $f(\boldsymbol{\theta}_t)$ has Lipschitz continuous gradient with parameter $L_f$ and the update rule $\boldsymbol{\theta}_{t+1} = \boldsymbol{\theta}_t - \eta \mathbf{g}_t$ we obtain
\begin{equation*}
	\begin{aligned}
	f(\boldsymbol{\theta}_{t+1}) - f(\boldsymbol{\theta}_{t}) 
	&\leq \langle \nabla f(\boldsymbol{\theta}_t), \boldsymbol{\theta}_{t+1}-\boldsymbol{\theta}_{t}\rangle + \frac{L_f}{2}\|\boldsymbol{\theta}_{t+1}-\boldsymbol{\theta}_{t}\|^2 \\
		& = -\eta \langle \nabla f(\boldsymbol{\theta}_t), \mathbf{g}_t \rangle + \frac{L_f}{2}\|\boldsymbol{\theta}_{t+1}-\boldsymbol{\theta}_{t}\|^2\\
		& = -\eta \langle \nabla f(\boldsymbol{\theta}_t), \nabla f(\boldsymbol{\theta}_t) - \nabla f(\boldsymbol{\theta}_t) + \mathbf{g}_t \rangle + \frac{L_f}{2}\|\boldsymbol{\theta}_{t+1}-\boldsymbol{\theta}_{t}\|^2\\
		& = -\eta \|\nabla f(\boldsymbol{\theta}_t)\|^2 - \eta \langle \nabla f(\boldsymbol{\theta}_t) , \mathbf{g}_t - \nabla f(\boldsymbol{\theta}_t)\rangle + \frac{\eta^2 L_f}{2}\|\mathbf{g}_t\|^2\\
	\end{aligned}
\end{equation*}

Plus and minus $\nabla f(\boldsymbol{\theta}_t)$ to $\mathbf{g}_t$ we have
\begin{equation*}
    \begin{aligned}
        \|\mathbf{g}_t\|^2 &= \|\mathbf{g}_t - \nabla f(\boldsymbol{\theta}_t) + \nabla f(\boldsymbol{\theta}_t)\|^2 \\
        &= \|\mathbf{g}_t - \nabla f(\boldsymbol{\theta}_t)\|^2 + \|\nabla f(\boldsymbol{\theta}_t)\|^2 + 2\langle \nabla f(\boldsymbol{\theta}_t) , \mathbf{g}_t-\nabla f(\boldsymbol{\theta}_t)\rangle
    \end{aligned}
\end{equation*}

Plug it back inside, we have
\begin{equation*}
	\begin{aligned}
	f(\boldsymbol{\theta}_{t+1}) - f(\boldsymbol{\theta}_{t}) 
	&\leq \left(\frac{\eta^2 L_f}{2}-\eta\right)\|\nabla f(\boldsymbol{\theta}_t)\|^2 + \left(\eta^2 L_f - \eta \right)\langle \nabla f(\boldsymbol{\theta}_t) , \mathbf{g}_t-\nabla f(\boldsymbol{\theta}_t)\rangle \\
	&\qquad + \frac{\eta^2 L_f}{2}\|\mathbf{g}_t-\nabla f(\boldsymbol{\theta}_t)\|^2
	\end{aligned}
\end{equation*}

Using the fact that $2\langle \nabla f(\boldsymbol{\theta}_t) , \mathbf{g}_t-\nabla f(\boldsymbol{\theta}_t)\rangle \leq \|\nabla f(\boldsymbol{\theta}_t)\|^2 + \|\mathbf{g}_t-\nabla f(\boldsymbol{\theta}_t)\|^2$, we have
\begin{equation*}
	\begin{aligned}
	f(\boldsymbol{\theta}_{t+1}) - f(\boldsymbol{\theta}_{t}) 
	&\leq \left(\eta^2 L_f-\frac{3}{2}\eta\right)\|\nabla f(\boldsymbol{\theta}_t)\|^2 + \left(\eta^2 L_f-\frac{1}{2}\eta\right) \|\mathbf{g}_t-\nabla f(\boldsymbol{\theta}_t)\|^2 \\
	\end{aligned}
\end{equation*}

Take expectation of both side and rearrange it we have
\begin{equation*}
    \begin{aligned}
    \left(\frac{3}{2}\eta - \eta^2 L_f\right)\cE[\|\nabla f(\boldsymbol{\theta}_t)\|^2] &\leq \cE[f(\boldsymbol{\theta}_{t})] - \cE[f(\boldsymbol{\theta}_{t+1})] + \left(\eta^2 L_f-\frac{1}{2}\eta\right) \Delta \\
    &\leq \cE[f(\boldsymbol{\theta}_{t})] - \cE[f(\boldsymbol{\theta}_{t+1})] + \eta^2 L_f \Delta
    \end{aligned}
\end{equation*}
where the last inequality hold when $\eta>0$.

Summing up from $t=1$ to $t=T$ on both side and using the fact that $f(\mathbf{w_*}) \leq f(\boldsymbol{\theta}_{t+1})$ we have
\begin{equation*}
	\begin{aligned}
	\left(\frac{3}{2}\eta - \eta^2 L_f\right) \sum_{t=1}^T \cE[\|\nabla f(\boldsymbol{\theta}_t)\|^2] \leq \cE[f(\boldsymbol{\theta}_{1})] - \cE[f(\boldsymbol{\theta}_{*})] + T \eta^2 L_f\Delta
	\end{aligned}
\end{equation*}

Divide both side by $T\left(\frac{3}{2}\eta - \eta^2 L_f\right)$ we have
\begin{equation*}
	\begin{aligned}
	\frac{1}{T}\sum_{t=1}^T \cE[\|\nabla f(\boldsymbol{\theta}_t)\|^2] &\leq \left(\frac{3}{2}\eta - \eta^2 L_f\right)^{-1} \frac{\left(\cE[f(\boldsymbol{\theta}_{1})] - \cE[f(\boldsymbol{\theta}_{*})]\right)}{T} + \Delta \frac{\left(2\eta^2 L_f\right)}{\left(3\eta - 2\eta^2 L_f\right)} \\
	&= \left(3\eta - 2\eta^2 L_f\right)^{-1} \frac{2\left(\cE[f(\boldsymbol{\theta}_{1})] - \cE[f(\boldsymbol{\theta}_{*})]\right)}{T} + \Delta \frac{\left(2\eta L_f\right)}{\left(3 - 2\eta L_f\right)} 
	\end{aligned}
\end{equation*}

Let $\eta = \min\{\frac{1}{L_f}, \sqrt{\frac{\cE[f(\boldsymbol{\theta}_{1})] - \cE[f(\boldsymbol{\theta}_{*})]}{\Delta L_f T}}\}$ we have
\begin{equation*}
	\begin{aligned}
	\frac{1}{T}\sum_{t=1}^T \cE[\|\nabla f(\boldsymbol{\theta}_t)\|^2] &\leq \frac{1}{\eta\left(3 - 2\eta L_f\right)} \frac{2\left(\cE[f(\boldsymbol{\theta}_{1})] - \cE[f(\boldsymbol{\theta}_{*})]\right)}{T} + \Delta \frac{\left(2\eta L_f\right)}{\left(3 - 2\eta L_f\right)} \\
	&\leq \frac{1}{\eta} \frac{2\left(\cE[f(\boldsymbol{\theta}_{1})] - \cE[f(\boldsymbol{\theta}_{*})]\right)}{T} + \Delta (2\eta L_f) \\
	&\leq \sqrt{\frac{16L_f \Delta \left(\cE[f(\boldsymbol{\theta}_{1})] - \cE[f(\boldsymbol{\theta}_{*})]\right)}{T}}% \leq \cO\left(\sqrt{\Delta/T}\right)
	\end{aligned}
\end{equation*}

Since $\Tilde{\boldsymbol{\theta}}$ is the minimum that less than the average, we have
\begin{equation*}
    \cE[\|f(\Tilde{\boldsymbol{\theta}})\|^2] \leq \sqrt{\frac{16L_f \Delta \left(\cE[f(\boldsymbol{\theta}_{1})] - \cE[f(\boldsymbol{\theta}_{*})]\right)}{T}}
\end{equation*}
\end{proof}

%#######################################
%#########Ignore Embedding Vars ########
\begin{remark}\label{remark:diff_g_tilde_g}
Note that due to the multi-level composition structure of stochastic GCNs, its stochastic gradient $\tilde{\mathbf{g}}$ is a biased estimation of full gradient $\nabla f(\boldsymbol{\theta})$, i.e., $\cE[\tilde{\mathbf{g}}] \neq \nabla f(\boldsymbol{\theta})$. To see this, 
let us formulate a $L$-layer GCN as a multi-level composite stochastic optimization problems of the form 
\begin{equation}\label{equation:sgcn}
    \min f(\boldsymbol{\theta}) = 
    \mathbb{E}_{\omega_L}\Big[ f_{\omega_L}^{(L)} \Big( 
    \mathbb{E}_{\omega_{L-1}}\big[ f_{\omega_{L-1}}^{(L-1)} \big( 
    \cdots 
    \mathbb{E}_{\omega_1} [ f_{\omega_1}^{(1)} ( \boldsymbol{\theta} )]
    \cdots
    \big) \big]
    \Big) \Big],
\end{equation}
where $\boldsymbol{\theta} = \{\mathbf{W}^{(1)},\cdots,\mathbf{W}^{(L)}\}$, random variable $\omega_\ell$ is a set of nodes stochastic GCN sampled at $\ell$-th layer. 

For the ease of presentation, let us denote $F^{(\ell)} := f^{(\ell)}\circ f^{(\ell-1)} \circ \cdots \circ f^{(1)}$.
By the chain rule, the full gradient is calculated as
\begin{equation*}
    \nabla f(\boldsymbol{\theta}) = \nabla f^{(1)}(\boldsymbol{\theta}) \cdot \nabla f^{(2)}(F^{(1)}(\boldsymbol{\theta})) \cdots \nabla f^{(L)}(F^{(L-1)}(\boldsymbol{\theta}))
\end{equation*}

For a given sample path $(\omega_1,\cdots,\omega_L)$, one may formulate an unbiased estimate of $\nabla f(\boldsymbol{\theta})$ as
\begin{equation*}
    \mathbf{g} = \nabla f_{\omega_1}^{(1)}(\boldsymbol{\theta}) \cdot \nabla f_{\omega_2}^{(2)}(F^{(1)}(\boldsymbol{\theta})) \cdots \nabla f_{\omega_L}^{(L)}(F^{(L-1)}(\boldsymbol{\theta}))
\end{equation*}
which cannot be calculated because $F^{(\ell)}(\boldsymbol{\theta}) = f^{(\ell)}\circ f^{(\ell-1)}\circ f^{(1)}(\boldsymbol{\theta})$ for $\ell\geq2$ are unfortunately not known.

As a result, when $L=1$, the objective function is linear in the distribution of the random variable $\omega$. For problem with $L\geq 2$, the nonlinear composition between expectations and component functions creates an objective function that is highly nonlinear with respect the the joint probability distribution $\omega_1, \cdots, \omega_L$.
In other word, the stochastic gradient $\tilde{\mathbf{g}}$ is a biased estimate of $\nabla f(\boldsymbol{\theta})$, where
\begin{equation*}
    \tilde{\mathbf{g}} := \nabla f^{(1)}_{\omega_1}(\boldsymbol{\theta}) \nabla f^{(2)}_{\omega_2}(f_{\omega_1}^{(1)}(\boldsymbol{\theta})) \cdots \nabla f^{(L)}_{\omega_L}(f_{\omega_{L-1}}^{(L-1)}\circ \cdots \circ f_{\omega_1}^{(1)}(\boldsymbol{\theta}))
\end{equation*}

Therefore, to analysis the convergence behavior of GCNs, we derivate the connections between $\mathbf{g}$, $\tilde{\mathbf{g}}$, and $\nabla f(\boldsymbol{\theta})$ in Lemma \ref{lemma:mse}.
\end{remark}

%#######################################
%#########Mean-square Error ############
\begin{lemma}\label{lemma:mse}
The mean square error of stochastic gradient estimator $\cE_t[\|\tilde{\mathbf{g}}_t - \nabla F(\boldsymbol{\theta}_t)\|]$ can be decomposed as
\begin{equation*}
    \cE_t[\|\tilde{\mathbf{g}}_t - \nabla F(\boldsymbol{\theta}_t)\|^2] = \cE_t[\|\tilde{\mathbf{g}}_t - \mathbf{g}_t\|^2] + \cE_t[\|\mathbf{g}_t - \nabla F(\boldsymbol{\theta}_t)\|^2],
\end{equation*}
where $\cE_t[\tilde{\mathbf{g}}_t] = \mathbf{g}_t$.
\end{lemma}
\begin{proof} [Proof of Lemma \ref{lemma:mse}]
\begin{equation*}
    \begin{aligned}
     \|\tilde{\mathbf{g}}_t - \nabla F(\boldsymbol{\theta}_t)\|^2 &= \|\tilde{\mathbf{g}}_t - \tilde{\mathbf{g}}_t + \mathbf{g}_t - \nabla F(\boldsymbol{\theta}_t)\|^2 \\
     &=\|\tilde{\mathbf{g}}_t - \mathbf{g}_t\|^2 + \|\mathbf{g}_t - \nabla F(\boldsymbol{\theta}_t)\|^2 + 2\langle\tilde{\mathbf{g}}_t - \mathbf{g}_t ,\mathbf{g}_t - \nabla F(\boldsymbol{\theta}_t)\rangle
    \end{aligned}
\end{equation*}

Take expectation on both side, using the fact that $\cE_t[\tilde{\mathbf{g}}_t] = \mathbf{g}_t$, we conclude the proof.
\end{proof}
%#######################################
%######### Bias ########################
\begin{lemma}\label{lemma:grad_bias}
Denote $\mathbb{V}_\ell$ as the upper-bound function approximation variance $\cE[\|f^{(\ell)}\circ \cdots \circ f^{(1)}(\boldsymbol{\theta}) - f_{\omega_\ell}^{(\ell)}\circ \cdots \circ f_{\omega_1}^{(1)}(\boldsymbol{\theta})\|^2]$. Then we have
\begin{equation*}
    \cE[\|\mathbf{g}-\tilde{\mathbf{g}}\|^2] \leq L\cdot\sum_{\ell=2}^L \left(\prod_{i=1}^{\ell-1} \rho^2_i \right)\left(\prod_{i=\ell+1}^L \rho^2_i \right) L^2_\ell \cdot \mathbb{V}_\ell
\end{equation*}
\end{lemma}
\begin{proof} [Proof of Lemma \ref{lemma:grad_bias}]
We can bound $\|\mathbf{g}-\tilde{\mathbf{g}}\|$ by add and subtract intermediate terms inside the such that each adjacent pair of products differ at most in one factor
\begin{equation*}
    \begin{aligned}
        \cE[\|\mathbf{g}-\tilde{\mathbf{g}}\|^2] &= \cE[\|\nabla f_{\omega_1}^{(1)}(\boldsymbol{\theta}_t) \cdot \nabla f_{\omega_2}^{(2)}(F^{(1)}(\boldsymbol{\theta})) \cdot \nabla f_{\omega_3}^{(2)}(F^{(2)}(\boldsymbol{\theta})) \cdots \nabla f_{\omega_L}^{(L)}(F^{(L-1)}(\boldsymbol{\theta})) \\
        &\qquad - \nabla f^{(1)}_{\omega_1}(\boldsymbol{\theta})\cdot \nabla f^{(2)}_{\omega_2}(f_{\omega_1}^{(1)}(\boldsymbol{\theta})) \cdot \nabla f_{\omega_3}^{(3)}(f_{\omega_2}^{(2)}\circ f_{\omega_1}^{(1)}(\boldsymbol{\theta})) \cdots \nabla f^{(L)}_{\omega_L}(f_{\omega_{L-1}}^{(L-1)}\circ \cdots \circ f_{\omega_1}^{(1)}(\boldsymbol{\theta}))\|^2] \\
        &\leq L\cdot(\cE[\|\nabla f_{\omega_1}^{(1)}(\boldsymbol{\theta}) \cdot \nabla f_{\omega_2}^{(2)}(F^{(1)}(\boldsymbol{\theta})) \cdot \nabla f_{\omega_3}^{(3)}(F^{(2)}(\boldsymbol{\theta})) \cdots \nabla f_{\omega_L}^{(L)}(F^{(L-1)}(\boldsymbol{\theta})) \\
        &\qquad - \nabla f^{(1)}_{\omega_1}(\boldsymbol{\theta}) \cdot \nabla f^{(2)}_{\omega_2}(f_{\omega_1}^{(1)}(\boldsymbol{\theta})) \cdot \nabla f_{\omega_3}^{(3)}(F^{(2)}(\boldsymbol{\theta})) \cdots \nabla f_{\omega_L}^{(L)}(F^{(L-1)}(\boldsymbol{\theta}))\|^2] \\
        &\quad + \cE[\|\nabla f^{(1)}_{\omega_1}(\boldsymbol{\theta}) \cdot \nabla f^{(2)}_{\omega_2}(f_{\omega_1}^{(1)}(\boldsymbol{\theta})) \cdot \nabla f_{\omega_3}^{(3)}(F^{(2)}(\boldsymbol{\theta})) \cdots \nabla f_{\omega_L}^{(L)}(F^{(L-1)}(\boldsymbol{\theta})) \\
        &\qquad - \nabla f^{(1)}_{\omega_1}(\boldsymbol{\theta}) \cdot \nabla f^{(2)}_{\omega_2}(f_{\omega_1}^{(1)}(\boldsymbol{\theta})) \cdot \nabla f_{\omega_3}^{(3)}(f_{\omega_2}^{(2)}\circ f_{\omega_1}^{(1)}(\boldsymbol{\theta})) \cdots \nabla f_{\omega_L}^{(L)}(F^{(L-1)}(\boldsymbol{\theta}))\|^2] +\cdots \\
        &\quad + \cE[\|\nabla f^{(1)}_{\omega_1}(\boldsymbol{\theta})\cdot \nabla f^{(2)}_{\omega_2}(f_{\omega_1}^{(1)}(\boldsymbol{\theta})) \cdot \nabla f_{\omega_3}^{(3)}(f_{\omega_2}^{(2)}\circ f_{\omega_1}^{(1)}(\boldsymbol{\theta})) \cdots \nabla f^{(L)}_{\omega_L}(F^{(L-1)}(\boldsymbol{\theta})) \\
        &\qquad - \nabla f^{(1)}_{\omega_1}(\boldsymbol{\theta})\cdot \nabla f^{(2)}_{\omega_2}(f_{\omega_1}^{(1)}(\boldsymbol{\theta})) \cdot \nabla f_{\omega_3}^{(3)}(f_{\omega_2}^{(2)}\circ f_{\omega_1}^{(1)}(\boldsymbol{\theta})) \cdots \nabla f^{(L)}_{\omega_L}(f_{\omega_{L-1}}^{(L-1)}\circ \cdots \circ f_{\omega_1}^{(1)}(\boldsymbol{\theta}))\|^2] ) \\
        &\leq L\cdot\sum_{\ell=2}^L \left(\prod_{i=1}^{\ell-1} \rho^2_i \right)\left(\prod_{i=\ell+1}^L \rho^2_i \right) L^2_\ell \cdot \mathbb{V}_\ell 
    \end{aligned}
\end{equation*}
where $\mathbb{V}_\ell$ is the upper-bound function approximation variance.
\end{proof}

\paragraph{Proof of Theorem \ref{theorem:sgcn_general_theorem}}
\begin{proof}
\todo{need update}
By Lemma \ref{lemma:mse}, and Lemma \ref{lemma:grad_diff} we have
\begin{equation*}
    \begin{aligned}
    \cE[\|\tilde{\mathbf{g}} - \nabla f(\boldsymbol{\theta})\|^2] &= \cE[\|\mathbf{g} - \nabla f(\boldsymbol{\theta})\|^2] + \cE[\|\tilde{\mathbf{g}} - \mathbf{g}\|^2]\\
    &\leq \cE[\|\mathbf{g} - \nabla f(\boldsymbol{\theta})\|^2] + L\cdot\sum_{\ell=1}^L \left(\prod_{i=1}^\ell \rho^2_i \right)\left(\prod_{i=\ell+1}^L \rho^2_i \right) L^2_\ell \cdot \mathbb{V}_\ell
    \end{aligned}
\end{equation*}

By Lemma \ref{lemma:is_vs_us}, we know that the variance of stochastic GCN gradient is bounded by $\tilde{\Delta}_{is}$ and $\tilde{\Delta}_{us}$ for minimal variance sampling and uniform sampling respectively 
\begin{equation*}
    \begin{aligned}
    \tilde{\Delta}_{is} &= \sum_{i=1}^n \frac{\|\nabla f_i(\boldsymbol{\theta})\|^2}{n} + L\cdot\sum_{\ell=1}^L \left(\prod_{i=1}^\ell \rho^2_i \right)\left(\prod_{i=\ell+1}^L \rho^2_i \right) L^2_\ell \cdot \mathbb{V}_\ell \\
    \tilde{\Delta}_{us} &= \left( \sum_{i=1}^n \frac{\|\nabla f_i(\boldsymbol{\theta})\|}{n} \right)^2 + L\cdot\sum_{\ell=1}^L \left(\prod_{i=1}^\ell \rho^2_i \right)\left(\prod_{i=\ell+1}^L \rho^2_i \right) L^2_\ell \cdot \mathbb{V}_\ell
    \end{aligned}
\end{equation*}

By Lemma \ref{lemma:convergence_rate_general}, we know that by using step size $\eta = \min\{\frac{1}{L_f}, \sqrt{\frac{\cE[f(\boldsymbol{\theta}_{1})] - \cE[f(\boldsymbol{\theta}_{*})]}{\tilde{\Delta} L_f T}}\}$ we have
\begin{equation*}
    \cE[\|\nabla f(\Tilde{\boldsymbol{\theta}}_t)\|^2] \leq \cO(\sqrt{\tilde{\Delta}/T}),
\end{equation*}
therefore conclude the proof.
\end{proof}
