# Supplementary material for: Minimal Variance Sampling with Provable Guarantees for Fast Training of Graph Neural Networks
Source: arXiv:2006.13866 source file (2021-09-05)
Supplement: Supplementary file 5 [file upper_bound_grad_norm.tex]

\section{Upper bound to the gradient norm}\label{appendix:upper_bound_grad_norm}
Let $\boldsymbol{\theta}=\{\mathbf{W}^{(1)},\cdots,\mathbf{W}^{(L)}\}$ be the weight matrices and $\sigma(\cdot)$ is the activation function. $L$-layer GCN can be write as
\begin{equation*}
    \begin{aligned}
    \mathbf{H}^{(0)} &= \mathbf{X} \\
    \mathbf{Z}^{(\ell)} &= \mathbf{L}^{(\ell)} \mathbf{H}^{(\ell-1)} \mathbf{W}^{(\ell)} \\
    \mathbf{H}^{(\ell)} &= \sigma(\mathbf{Z}^{(\ell)}) \\
    \end{aligned}
\end{equation*}

We define the gradient of the loss with respect to the output of the network as
\begin{equation*}
    \nabla_{\mathbf{Z}_i^{(L)}} \mathcal{L} = \nabla_{\mathbf{Z}_i^{(L)}} \mathcal{L}(\mathbf{Z}_i^{(L)}, y_i)
\end{equation*}
and the gradient of the loss with respect to the output of layer $\ell$ as \begin{equation*}
    \nabla_{\mathbf{Z}_i^{(\ell)}} \mathcal{L} = \Delta_i^{(\ell)} \sigma'(\mathbf{Z}_i^{(L)}) \nabla_{\mathbf{H}_i^{(L)}} \mathcal{L},
\end{equation*}
where 
\begin{equation*}\begin{aligned}
\Delta_i^{(\ell)} = \sigma'(\mathbf{Z}_i^{(\ell)}) \mathbf{L}^{(\ell+1)} \mathbf{W}^{(\ell+1)} \dots \sigma'(\mathbf{Z}_i^{(L-1)}) \mathbf{L}^{(L)} \mathbf{W}^{(L)}
\end{aligned}\end{equation*}

Finally, the gradient with respect to the parameters of the $\ell$-th layer can be written
\begin{equation*}
    \begin{aligned}
        \|\nabla_{\mathbf{W}^{(\ell)}} \mathcal{L}\|_2 &= \| \Delta_i^{(\ell)} \sigma'(\mathbf{Z}_i^{(L)}) \nabla_{\mathbf{H}_i^{(L)}}\mathcal{L} \cdot \mathbf{L}^{(\ell-1)} \mathbf{H}_i^{(\ell-1)}\|_2 \\
        &\leq \|\mathbf{L}_i^{(\ell-1)}\mathbf{H}_i^{(\ell-1)}\|_2 \|\Delta_i^{(\ell)}\|_2 \|\sigma'(\mathbf{Z}_i^{(L)}) \nabla_{\mathbf{H}_i^{(L)}} \mathcal{L}\|_2
    \end{aligned}
\end{equation*}

We observe that $\mathbf{H}_i^{(\ell)}$ and $\Delta_i^{(\ell)}$ depend only on $\mathbf{Z}_i$ and $\boldsymbol{\theta}$. However, due to various weight initialization and activation normalization techniques those quantities do not capture the important per sample variations of the gradient norm. Therefore, we can deduce the following upper bound per layer
\begin{equation*}
    \begin{aligned}
    \|\nabla_{\mathbf{W}^{(\ell)}} \mathcal{L}\|_2 &= \max_{\ell, i} \left( \|\mathbf{L}_i^{(\ell-1)} \mathbf{H}_i^{(\ell-1)}\|_2 \|\Delta_i^{(\ell)}\|_2\right) \|\sigma'(\mathbf{Z}_i^{(L)}) \nabla_{\mathbf{H}_i^{(L)}} \mathcal{L}\|_2 \\
    &= \rho \|\sigma'(\mathbf{Z}_i^{(L)}) \nabla_{\mathbf{H}_i^{(L)}} \mathcal{L}\|_2
    \end{aligned}
\end{equation*}
which can then be used to derive our final upper bound
\begin{equation*}\begin{aligned}
    \| \nabla_{\boldsymbol{\theta}} \mathcal{L} \|_2 \leq
        \underbrace{L \rho \|\sigma'(\mathbf{Z}_i^{(L)})
            \nabla_{\mathbf{H}_i^{(L)}}\mathcal{L}\|_2}_{\hat{G}_i} \label{eq:sup_upper_bound}.
\end{aligned}\end{equation*}

Intuitively, the above means that the variations of the gradient norm are mostly captured by the final classification layer. Consequently, we can use the gradient of the loss with respect to the pre-activation outputs of our neural network as an upper bound to the per-sample gradient norm.
